# Supplementary material for: Bridging Time and Space: Decoupled Spatio-Temporal Alignment for Video Grounding
Source: arXiv:2604.08014 source file (2026-11-19)
Supplement: Supplementary file 1 [file Appendix.tex]

%%
%% This is file `sample-sigconf-authordraft.tex',
%% generated with the docstrip utility.
%%
%% The original source files were:
%%
%% samples.dtx  (with options: `all,proceedings,bibtex,authordraft')
%% 
%% IMPORTANT NOTICE:
%% 
%% For the copyright see the source file.
%% 
%% Any modified versions of this file must be renamed
%% with new filenames distinct from sample-sigconf-authordraft.tex.
%% 
%% For distribution of the original source see the terms
%% for copying and modification in the file samples.dtx.
%% 
%% This generated file may be distributed as long as the
%% original source files, as listed above, are part of the
%% same distribution. (The sources need not necessarily be
%% in the same archive or directory.)
%%
%%
%% Commands for TeXCount
%TC:macro \cite [option:text,text]
%TC:macro \citep [option:text,text]
%TC:macro \citet [option:text,text]
%TC:envir table 0 1
%TC:envir table* 0 1
%TC:envir tabular [ignore] word
%TC:envir displaymath 0 word
%TC:envir math 0 word
%TC:envir comment 0 0
%%
%% The first command in your LaTeX source must be the \documentclass
%% command.
%%
%% For submission and review of your manuscript please change the
%% command to \documentclass[manuscript, screen, review]{acmart}.
%%
%% When submitting camera ready or to TAPS, please change the command
%% to \documentclass[sigconf]{acmart} or whichever template is required
%% for your publication.
%%
%%
% \documentclass[sigconf,authordraft]{acmart}
\documentclass[sigconf, screen, review, anonymous]{acmart}

\settopmatter{printacmref=false} % Removes citation information below abstract
\renewcommand\footnotetextcopyrightpermission[1]{} % removes footnote with conference information in first column
\pagestyle{plain} % removes running headers

\usepackage{enumitem}
\usepackage{makecell}
\usepackage{tabulary}
\usepackage[table]{xcolor}
\usepackage{colortbl}
\usepackage{multirow}
\usepackage{tabularx}
\usepackage{array}
\usepackage{graphicx}
\newcolumntype{Y}{>{\centering\arraybackslash\hspace{0pt}\nohyphens}X}
\usepackage{stfloats}
\definecolor{shallowblue}{RGB}{227, 240, 249}
\definecolor{deepblue}{RGB}{192, 216, 240}
%%
%% \BibTeX command to typeset BibTeX logo in the docs
\AtBeginDocument{%
  }

%% Rights management information.  This information is sent to you
%% when you complete the rights form.  These commands have SAMPLE
%% values in them; it is your responsibility as an author to replace
%% the commands and values with those provided to you when you
%% complete the rights form.
\setcopyright{acmlicensed}
\copyrightyear{2018}
\acmYear{2018}
\acmDOI{XXXXXXX.XXXXXXX}
%% These commands are for a PROCEEDINGS abstract or paper.
% \acmConference[Conference acronym 'XX]{Make sure to enter the correct
%   conference title from your rights confirmation email}{June 03--05,
%   2018}{Woodstock, NY}
%%

\acmConference[MM '26]{Make sure to enter the correct
  conference title from your rights confirmation email}{November 10–-14,
  2026}{Rio de Janeiro, Brazil}
%%  Uncomment \acmBooktitle if the title of the proceedings is different
%%  from ``Proceedings of ...''!
%%
%%\acmBooktitle{Woodstock '18: ACM Symposium on Neural Gaze Detection,
%%  June 03--05, 2018, Woodstock, NY}
\acmISBN{978-1-4503-XXXX-X/2018/06}

%%
%% Submission ID.
%% Use this when submitting an article to a sponsored event. You'll
%% receive a unique submission ID from the organizers
%% of the event, and this ID should be used as the parameter to this command.
%%\acmSubmissionID{123-A56-BU3}

%%
%% For managing citations, it is recommended to use bibliography
%% files in BibTeX format.
%%
%% You can then either use BibTeX with the ACM-Reference-Format style,
%% or BibLaTeX with the acmnumeric or acmauthoryear sytles, that include
%% support for advanced citation of software artefact from the
%% biblatex-software package, also separately available on CTAN.
%%
%% Look at the sample-*-biblatex.tex files for templates showcasing
%% the biblatex styles.
%%

%%
%% The majority of ACM publications use numbered citations and
%% references.  The command \citestyle{authoryear} switches to the
%% "author year" style.
%%
%% If you are preparing content for an event
%% sponsored by ACM SIGGRAPH, you must use the "author year" style of
%% citations and references.
%% Uncommenting
%% the next command will enable that style.
%%\citestyle{acmauthoryear}

%%
%% end of the preamble, start of the body of the document source.
\begin{document}

%%
%% The "title" command has an optional parameter,
%% allowing the author to define a "short title" to be used in page headers.
\title[Bridging Time and Space: Decoupled Spatio-Temporal Alignment for Video Grounding]{Bridging Time and Space: Decoupled Spatio-Temporal Alignment for Video Grounding\\Supplementary Material}

\maketitle

\appendix
\section{Self-Collected Data Details}
\label{appendix:data}
The self-collected data is synthesized from the REVOS~\cite{yan2024visa} video object segmentation dataset to augment STVG training diversity.
We choose to augment the ReVOS datasets is because they provide densely annotated mask sequences with object captions, bounding boxes, and temporal spans across a wide range of real-world video scenarios.

\subsection{Construction Pipeline}
Since REVOS annotations cover the full video duration rather than event-specific temporal windows, we cannot directly use them as STVG samples.
To address this, we construct the following pipeline:

(1) \textit{Bounding box extraction}:
We convert instance-level mask annotations into bounding boxes by computing their maximal enclosing regions, getting per-frame spatial coordinates.

(2) \textit{Temporal boundary generation}: 
Due to the masks span the full video, we insert semantically irrelevant video clips at the beginning or end of each sequence to generate timestamp boundaries, creating realistic temporal localization samples.

(3) \textit{Sample assembly}: 
Each synthetic sample is assembled with the object caption as the language query, the constructed bounding boxes as spatial ground truth, and the inserted temporal boundaries as the temporal grounding target.

\subsection{Quality Filtering}
To ensure data quality, we drops samples with videos longer than 180 seconds or annotation spans shorter than 1 second.
Because these videos represent either excessively long sequences that are difficult to process or near-degenerate temporal annotations.
After filtering, approximately 10K high-quality samples are retained.

\subsection{Role in Training}
The synthetic dataset serves as an effective STVG data augmentation source, enhancing the model's temporal grounding diversity.
By incorporating varied video domains and object categories from REVOS, it strengthens Bridge-STG's ability to generalize to open-vocabulary and complex real-world scenarios.
The self-collected dataset will be made publicly available alongside the code and model weights upon paper acceptance.

\section{Additional Experiments Details}
\subsection{Datasets}
\noindent\textbf{VidSTG}~\cite{zhang2020does} is a large-scale STVG benchmark built upon the VidOR video relation dataset, containing 10,000 videos split into 7,000/835/2,165 for training, validation, and testing.                                 
Each video is paired with both declarative and interrogative natural language queries, requiring the model to localize the referred object as a spatio-temporal tube.                                                                                 
The inclusion of interrogative sentences---which require implicit reasoning about video content to identify the target---makes VidSTG particularly challenging and representative of real-world grounding demands.

\noindent\textbf{HC-STVG}~\cite{tang2021human} (Human-Centric Spatio-Temporal Video Grounding) focuses on localizing specific persons in multi-person video scenarios.         
HC-STVG-v1 contains 5,660 video-sentence pairs with videos normalized to 20 seconds, while HC-STVG-v2 extends the benchmark with additional samples and refined annotations.                                                            
The dataset is constructed through a rigorous five-stage annotation pipeline to ensure quality and complexity, with an average ground-truth tube duration of 5.37 seconds.                                                                        
The human-centric nature and multi-person scenes make it a demanding benchmark for fine-grained spatio-temporal understanding.  

\noindent\textbf{Charades-STA}~\cite{gao2017tall} is a widely-used benchmark for Video Temporal Grounding (VTG), built upon the Charades dataset of indoor daily activities.
It contains 16,128 sentence-segment pairs (12,408 training / 3,720 testing), where each pair associates a natural language description with a temporal interval in the video.
Unlike STVG, Charades-STA requires only temporal localization without spatial grounding, making it a standard benchmark for evaluating temporal reasoning capabilities.

\noindent\textbf{GOT-10K}~\cite{huang2019got} is a large-scale benchmark for generic Visual Object Tracking (VOT), comprising over 10,000 video segments with more than 1.5 million manually labeled bounding boxes spanning 563 object classes and 87 motion patterns.
A key feature of GOT-10K is its one-shot evaluation protocol, where training and test object classes are strictly non-overlapping, ensuring unbiased assessment of generalization to unseen categories.

\noindent\textbf{RefCOCO / RefCOCO+ / RefCOCOg}~\cite{kazemzadeh2014referitgame, mao2016generation} are standard benchmarks for Referring Expression Comprehension (REC) on static images from MS COCO.
  RefCOCO contains $\sim$19,585 images with short, position-aware referring expressions; RefCOCO+ ($\sim$19,994 images) excludes spatial relationship words, requiring appearance-based
  discrimination; RefCOCOg ($\sim$26,711 images) features longer and more complex expressions.
  Each benchmark provides train/val/testA/testB splits, where testA and testB evaluate on images with multiple people and multiple objects, respectively.

\noindent\textbf{Video-MME}~\cite{fu2025video} is the first comprehensive evaluation benchmark for multi-modal LLMs in video analysis, containing 900 videos totaling over 254 hours across six visual domains.
It provides 2,700 expert-annotated question-answer pairs covering diverse temporal ranges and video types, with optional subtitle information.
We report accuracy both with and without subtitles to assess the model's video comprehension under different input conditions.

\subsection{Evaluation Metrics}
\noindent\textbf{m\_tIoU} (mean temporal IoU) measures the average Intersection-over-Union between predicted and ground-truth temporal intervals across all test queries:
\begin{equation}
\text{m\_tIoU} = \frac{1}{N}\sum_{i=1}^{N} \frac{|\hat{T}_i \cap T_i|}{|\hat{T}_i \cup T_i|},
\end{equation}
where $\hat{T}_i$ and $T_i$ denote the predicted and ground-truth temporal intervals for the $i$-th query, respectively. This metric evaluates the quality of temporal boundary prediction independently of spatial localization.

\noindent\textbf{m\_vIoU} (mean video IoU) extends temporal IoU to the full spatio-temporal tube by averaging the per-frame spatial IoU over the union of predicted and ground-truth temporal intervals:
\begin{equation}
\text{m\_vIoU} = \frac{1}{N}\sum_{i=1}^{N} \frac{1}{|\hat{T}_i \cup T_i|} \sum_{t \in \hat{T}_i \cup T_i} \text{IoU}(\hat{b}_i^t, b_i^t),
\end{equation}
where $\hat{b}_i^t$ and $b_i^t$ are the predicted and ground-truth bounding boxes at frame $t$. Frames outside the ground-truth interval contribute zero IoU. m\_vIoU jointly evaluates temporal and spatial grounding, making it the primary metric for STVG.

\noindent\textbf{vIoU@R} measures the proportion of test queries whose m\_vIoU exceeds a threshold $R$:
\begin{equation}
\text{vIoU@}R = \frac{1}{N}\sum_{i=1}^{N} \mathbf{1}[\text{vIoU}_i \geq R].
\end{equation}
We report vIoU@0.3 and vIoU@0.5, where the latter imposes a stricter localization requirement.

\noindent\textbf{R@1 IoU=$\tau$} for VTG measures the percentage of queries where the top-1 predicted temporal segment achieves IoU $\geq \tau$ with the ground truth. We report R@1 at $\tau \in \{0.5, 0.7\}$ on Charades-STA.

\noindent\textbf{AO, SR$_{0.5}$, SR$_{0.75}$} for VOT follow the GOT-10K protocol~\cite{huang2019got}. AO (Average Overlap) is the mean IoU across all frames in all test sequences. 
SR$_{0.5}$ and SR$_{0.75}$ (Success Rate) measure the percentage of frames where IoU exceeds 0.5 and 0.75, respectively.

\noindent\textbf{IoU@0.5} for REC measures the percentage of referring expressions where the predicted bounding box achieves IoU $\geq 0.5$ with the ground truth, following standard practice in visual grounding evaluation.

\subsection{QGSL Architecture Details}
For reproducibility, we provide the detailed architecture of the Query-Guided Spatial Localization (QGSL) module. QGSL is built based on the OV-DINO~\cite{wang2024ov} framework, which uses:                  
             
\begin{itemize}[leftmargin=*,nosep]                                                                    
    \item \textbf{Image Backbone}: Swin Transformer-Large pretrained on COCO.      
    \item \textbf{Image Encoder}: 6-layer feature pyramid network with deformable attention.             
    \item \textbf{Spatial Decoder}: 6-layer Deformable DETR-style decoder~\cite{zhu2020deformable} with deformable cross-attention between object queries and multi-scale image features.                    
    \item \textbf{Training Supervision}: Hungarian-algorithm-based bipartite matching between predicted boxes and ground-truth annotations, with standard detection losses ($\mathcal{L}_{obj}$, $\mathcal{L}_{box}$, $\mathcal{L}_{giou}$). 
\end{itemize}                                                                                            Additionally, the text backbone in the original OV-DINO is removed. 

\subsection{Gradient Flow and Parameter Update}
In this subsection, we describe which parameters are updated by each loss term. 
$\mathcal{L}_{token}$ (Eq.~7 in the main paper) supervises the MLLM's autoregressive output and updates only the LoRA adapters~\cite{hu2022lora} applied to the language tower of Qwen3-VL, including the self-attention projection matrices. 
The vision tower parameters remain frozen throughout training.  

$\mathcal{L}_{spatial}$ (Eq.~8 in the main paper) supervises the spatial grounding stage and updates all parameters of the QGSL module (image backbone, encoder, and decoder).              
Crucially, gradients from $\mathcal{L}_{spatial}$ also flow back through the bridging queries $\mathbf{Q}_{bridge}$ into the MLLM's LoRA adapters via the STSB mechanism (Eq.~3), enabling  end-to-end joint optimization.
No stop-gradient operation is applied at the STSB interface, allowing the spatial grounding signal to refine the MLLM's temporal reasoning context.

\subsection{ETA Compatibility with Qwen3-VL}
The Explicit Temporal Alignment (ETA) strategy (Eq.~1 in the main paper) assigns timestamp tokens to virtual spatial coordinates $(W+s, H+s)$ outside the visual token grid. 
In Qwen3-VL~\cite{bai2025qwen3}, the vision encoder applies a patch merger that reduces the spatial resolution of visual tokens.

Specifically, for an input video frame of resolution $H_{img} \times W_{img}$, the post-merger visual token grid has dimensions $H = \lfloor H_{img}/P \rfloor$ and $W = \lfloor W_{img}/P \rfloor$, where $P$ is the effective patch size after merging (typically $P=14$ for Qwen3-VL).                       
The virtual coordinates $(W+s, H+s)$ are computed based on this post-merger grid size, ensuring that timestamp tokens consistently fall outside the visual token occupancy region regardless of input resolution. 

\section{Inference Complexity Analysis}
 \label{appendix:complexity}
\begin{table*}[t]
\centering
\small
\setlength{\tabcolsep}{1pt}
\caption{Inference cost evaluation on VidSTG\_Declarative (100 samples). All data is average value, SpaceVLLM is not open-source.}
\label{tab:inference}
\begin{tabularx}{\linewidth}{>{\raggedright\arraybackslash}X*{11}{c}}
\hline
Model & \makecell{Num of\\parameters} & \makecell{Peak GPU\\memory} & \makecell{Video\\FPS} & \makecell{MLLM input\\tokens} & \makecell{Num of\\video frame} & \makecell{Video\\resolution} & \makecell{Num of MLLM\\generated token} & \makecell{Frames for\\spatial decoder} & \makecell{MLLM inference \\ time (ms/sample)} & \makecell{QGSL inference \\time (ms/sample)} \\
\hline
LLaVA-ST & 8095.71M & 31.4G & 14.96 & 2585.23 & 100 & 384*384 & 374.76 & - & 6685.31 & -\\
\hline
\rowcolor[gray]{0.9}
Bridge-STG & 8977.16M & \textbf{30.1G} & 24.20 & 4226.7 & 45.56 & 370.44*523.04 & \textbf{42.83} & 20.77 & \textbf{1671.92} & 210.39 \\
\hline
\end{tabularx}
\end{table*}

Bridge-STG is trained on 8 NVIDIA H100 GPUs for a total of 16.4 hours, which is comparable to standard MLLM fine-tuning pipelines of similar scale. 
Though the additional QGSL spatial decoder increases the total number of trainable parameters, the training cost overhead relative to the MLLM baseline is small.
This is because the decoder operates only on a small subset of frames rather than the full video.
Tab.~\ref{tab:inference} shows a detailed inference cost comparison between Bridge-STG and LLaVA-ST on 100 VidSTG declarative samples. We analyze the results from four perspectives. 

\subsection{Token Efficiency}                                                                      The most significant advantage of our decoupled design lies in LLM output token reduction.               LLaVA-ST generates an average of 374.76 tokens per sample to autoregressively produce bounding box coordinates for every frame, whereas Bridge-STG generates only 42.83 tokens—an \textbf{88.6\%} reduction.
This is because Bridge-STG delegates spatial localization to the QGSL decoder, requiring the MLLM to output only temporal boundary tokens rather than dense per-frame coordinates.
As a consequence, the MLLM inference latency drops from 6685.31 ms to 1671.92 ms (\textbf{75.0\%} reduction).              

\subsection{Frame Efficiency}                                                                      Bridge-STG processes an average of 45.56 video frames per sample, compared to 100 frames for LLaVA-ST.   This reduction is achieved by our P/N Frame Sampling strategy, which selects only the most discriminative positive and negative frames for spatial decoding.                                
Among these, an average of 20.77 frames are forwarded to the spatial decoder, further concentrating computation on the most informative content. 
Additionally, Bridge-STG preserves the original video aspect ratio (average 370$\times$523) rather than forcing a fixed 384$\times$384 resolution, which avoids spatial distortion in non-square videos.                

\subsection{Memory Efficiency.} 
Despite introducing the additional QGSL spatial decoder (resulting in a slightly larger parameter), Bridge-STG achieves a \textbf{lower} peak GPU memory usage (30.1G vs. 31.4G).
This is attributable to the reduced number of processed frames and the substantially shorter MLLM output sequence, both of which reduce the KV-cache and activation memory footprint during inference.

\subsection{Overall Latency.}
Including the QGSL spatial decoder (210.39 ms/sample), Bridge-STG's total inference time is 1882.31 ms/sample, which is \textbf{3.6$\times$ faster} than LLaVA-ST (6685.31 ms/sample).
These results demonstrate that the decoupled architecture not only improves grounding accuracy but also yields substantial practical efficiency gains, making Bridge-STG more suitable for real-world deployment.                              
 
\section{Additional Ablation Results}
This section provides supplementary ablation studies that complement the main paper.
All experiments are conducted on the declarative sentences subset of VidSTG~\cite{zhang2020does} using the same evaluation protocol as the main paper.

\subsection{Effect of ETA Virtual Coordinate Design}
The ETA module injects text-formatted timestamps into the MLLM's embedding space by assigning each timestamp token a virtual spatial coordinate $(W+s, H+s)$ outside the visual token grid.
This design preserves the coherence of the spatio-temporal positional embedding space while explicitly anchoring each timestamp to its corresponding visual content.
A natural question is whether this virtual coordinate placement is necessary, or whether naively appending timestamp tokens (without positional offset) achieves comparable results.

\begin{table}[h]
\centering
\setlength{\tabcolsep}{4pt}
\caption{Ablation on ETA timestamp injection strategy on VidSTG declarative subset.}
\label{tab:eta_ablation}
\begin{tabularx}{\linewidth}{>{\raggedright\arraybackslash}Xcccc}
\toprule
% \rowcolor[gray]{0.95}
ETA Design & m\_tIoU & m\_vIoU & vIoU@0.3 & vIoU@0.5 \\
\midrule
w/o ETA & 50.2 & 32.3 & 44.9 & 30.8 \\
Naive append & 51.4 & 35.8 & 49.6 & 36.1 \\
\rowcolor[gray]{0.9}
\textbf{Virtual coord. (Default)} & \textbf{52.6} & \textbf{37.2} & \textbf{52.4} & \textbf{37.4} \\
\bottomrule
\end{tabularx}
\end{table}

As shown in Tab.~\ref{tab:eta_ablation}, the virtual coordinate design consistently outperforms naive appending.
Without any positional offset, the injected timestamp tokens disrupt the MLLM's continuous positional embedding space, causing interference with adjacent visual tokens.
In contrast, placing timestamps at virtual coordinates $(W+s, H+s)$ keeps them spatially separated from the visual token grid, allowing the MLLM to treat them as structured temporal anchors without corrupting the visual feature representations.

\subsection{Effect of QGSL Encoder Layer Number}
The QGSL module uses an $n$-layer image encoder to produce hierarchical feature representations, with $n=6$ as the default setting (noted in Sec.~3.3 of the main paper).
Tab.~\ref{tab:encoder_layer} reports performance under different values of $n$.

\begin{table}[h]
\centering
\setlength{\tabcolsep}{4pt}
\caption{Ablation on the number of QGSL encoder layers $n$ on VidSTG declarative subset.}
\label{tab:encoder_layer}
\begin{tabularx}{\linewidth}{>{\raggedright\arraybackslash}Xcccc}
\toprule
% \rowcolor[gray]{0.95}
Encoder Layers $n$ & m\_tIoU & m\_vIoU & vIoU@0.3 & vIoU@0.5 \\
\midrule
$n=2$ & 52.6 & 34.2 & 46.4 &34.6\\
$n=4$ & 52.6 & 36.3 & 50.7 & 36.5 \\
\rowcolor[gray]{0.9}
$\mathbf{n=6}$ \textbf{(Default)} & \textbf{52.6} & \textbf{37.2} & \textbf{52.4} & \textbf{37.4} \\
$n=8$ & 52.6 & 36.9 & 51.4 & 37.0 \\
\bottomrule
\end{tabularx}
\end{table}

Fewer encoder layers limit the model's ability to build hierarchical spatial representations, reducing spatial grounding precision.
Conversely, increasing $n$ beyond 6 yields diminishing returns while adding computational overhead.
The default $n=6$ strikes the best balance between representational capacity and efficiency.
Notably, the number of encoder layers affects only spatial grounding metrics (m\_vIoU, vIoU@R) while leaving m\_tIoU unchanged, which is expected since temporal localization is performed entirely by the MLLM prior to QGSL. 
  
\subsection{Effect of Multi-Layer Query Aggregation}
Our QGSL module aggregates candidate queries from all $n$ encoder layers (Multi-Layer Interactive Queries), rather than selecting only from the final encoder layer as in standard detection frameworks.
Tab.~\ref{tab:multilayer} validates this design choice.

\begin{table}[h]
\centering
\setlength{\tabcolsep}{4pt}
\caption{Ablation on multi-layer vs. single-layer query selection in QGSL on VidSTG declarative subset.}
\label{tab:multilayer}
\begin{tabularx}{\linewidth}{>{\raggedright\arraybackslash}Xcccc}
\toprule
% \rowcolor[gray]{0.95}
Query Selection & m\_tIoU & m\_vIoU & vIoU@0.3 & vIoU@0.5 \\
\midrule
Single-layer (last) & 52.6 & 34.6 & 46.8 & 34.9 \\
\rowcolor[gray]{0.9}
\textbf{Multi-layer (Default)} & \textbf{52.6} & \textbf{37.2} & \textbf{52.4} & \textbf{37.4} \\
\bottomrule
\end{tabularx}
\end{table}

Relying solely on the last encoder layer discards fine-grained spatial features encoded in intermediate layers, which are critical for localizing small or partially occluded objects.
Multi-layer aggregation captures both low-level spatial details and high-level semantic representations, leading to more robust spatial grounding.
Similarly, the query selection strategy influences spatial grounding precision without affecting temporal localization, consistent with the decoupled nature of our architecture.

\subsection{Effect of Contrastive Image-Query Alignment} 
The contrastive alignment loss $\mathcal{L}_{align}$ (Eq.~6 in the main paper)  supervises the query selection process by pulling selected image features toward the bridging queries while pushing away unselected tokens. 
To validate its contribution, we ablate this loss by setting $\eta=0$ in Eq.~7.  
As shown in Tab.~\ref{tab:align_ablation}, removing $\mathcal{L}_{align}$ leads to a noticeable drop in spatial grounding performance (m\_vIoU decreases by 2.2), while temporal localization remains largely unaffected.       

\begin{table}[h] 
\centering     
\small     
\setlength{\tabcolsep}{4pt}  
\caption{Ablation on the contrastive alignment loss on VidSTG declarative subset.}
\label{tab:align_ablation}                                                                               
\begin{tabularx}{\linewidth}{>{\raggedright\arraybackslash}Xcccc}                                        
\toprule                                                                                                 
% \rowcolor[gray]{0.95}                                                                                    
Setting & m\_tIoU & m\_vIoU & vIoU@0.3 & vIoU@0.5 \\                                                     
\midrule                                                                                                 
w/o $\mathcal{L}_{align}$ & 52.6 & 35.0 & 48.5 & 35.2 \\                                                        
\rowcolor[gray]{0.9}                                                                                     
\textbf{With $\mathcal{L}_{align}$ (Default)} & \textbf{52.6} & \textbf{37.2} & \textbf{52.4} & \textbf{37.4} \\                                                                            
\bottomrule                                                                                              
\end{tabularx}                                                                                           
\end{table}

\subsection{Oracle Temporal Window Analysis}
To quantify the upper bound of Bridge-STG's spatial grounding capability and analyze the impact of temporal prediction errors, we replace the predicted temporal window with ground-truth annotations at inference time (``Oracle'' setting).

As shown in Tab.~\ref{tab:oracle}, the Oracle setting yields m\_vIoU of 65.2, compared to 37.2 under standard inference.
This gap reflects the inherent challenge of temporal localization in STVG, which is shared across all methods.
Importantly, Bridge-STG already achieves the highest temporal accuracy among all compared methods (m\_tIoU = 52.6), and the QGSL module maintains strong spatial grounding even under imperfect temporal windows---as evidenced by the 37.2 m\_vIoU achieved with predicted boundaries that are not perfectly aligned. 
The Oracle result further demonstrates that the QGSL spatial decoder itself has strong localization capacity, and that continued improvement in temporal prediction will directly translate to spatial grounding gains.

\begin{table}[h]
\centering
\small
\caption{Oracle temporal window experiment on VidSTG declarative subset.}
\label{tab:oracle}
\begin{tabularx}{\linewidth}{>{\raggedright\arraybackslash}Xcccc}
\toprule
% \rowcolor[gray]{0.95}
Setting & m\_tIoU & m\_vIoU & vIoU@0.3 & vIoU@0.5 \\
\midrule
Bridge-STG (Predicted) & 52.6 & 37.2 & 52.4 & 37.4 \\
\rowcolor[gray]{0.9}
Bridge-STG (Oracle GT) & --- & 65.2 & 73.2 & 59.3 \\
\bottomrule
\end{tabularx}
\end{table}

\subsection{Sensitivity of Spatial Grounding to Temporal Prediction Quality} 
To further characterize the relationship between temporal prediction quality and spatial grounding performance, we partition the VidSTG declarative set into four bins based on the predicted temporal IoU (tIoU) and report the corresponding m\_vIoU for each bin.        

\begin{table}[h]  
\centering  
\setlength{\tabcolsep}{8pt}
\caption{Spatial grounding performance (m\_vIoU) across temporal prediction quality bins on VidSTG declarative subset.}                                                                     
\label{tab:tiou_bin} 
\begin{tabularx}{\linewidth}{>{\raggedright\arraybackslash}Xccc}
\toprule
% \rowcolor[gray]{0.95} 
tIoU Bin & \#Samples & Avg.\ tIoU & m\_vIoU \\ 
\midrule 
$[0.0, 0.3)$  & 1556  & 7.0 & 4.2 \\
$[0.3, 0.5)$  & 453  & 38.0 & 24.5 \\ 
$[0.5, 0.7)$  & 686 & 57.8 & 38.5 \\
$[0.7, 1.0]$  & 1914 & 91.2 & 66.5\\
\midrule
\rowcolor[gray]{0.9}  
\textbf{Overall} & \textbf{4609} & \textbf{0.53} & \textbf{37.2} \\ 
\bottomrule 
\end{tabularx} 
\end{table}                                                                                                                                                                                 
As shown in Tab.~\ref{tab:tiou_bin}, spatial grounding performance exhibits positive correlation with temporal prediction quality.  
When the predicted temporal window achieves tIoU $\geq 0.7$ (41.5\% of test samples), QGSL attains 66.5 m\_vIoU.
In the moderate range $[0.5, 0.7)$, m\_vIoU remains strong at 38.5, demonstrating that QGSL can effectively leverage partially overlapping temporal windows to produce accurate spatial grounding.
Even at $[0.3, 0.5)$, the spatial decoder still achieves 24.5 m\_vIoU, confirming that moderate temporal overlap provides sufficient positive frames for meaningful localization.
Only when tIoU falls below 0.3 (33.8\% of samples) does spatial performance degrade severely to 4.2 m\_vIoU, since QGSL receives almost no positive frames.
These results demonstrate that cascade dependency is not catastrophic in practice: for the 66.2\% of test samples where tIoU $\geq 0.3$, the spatial decoder could produce valid and competitive grounding outputs.       
Furthermore, since Bridge-STG achieves the highest temporal localization accuracy among all compared methods (m\_tIoU = 52.6, Table~2 in the main paper), the proportion of low-tIoU failure cases is minimized relative to competing approaches.

\section{Performance on Edge Cases}
To better understand the boundary conditions of Bridge-STG, we evaluate its performance on two challenging edge cases from the VidSTG test set: videos with extreme durations and events with very short temporal spans. 

\begin{table*}[h]                                                                                         \centering                                                            
\setlength{\tabcolsep}{12pt}                                                                             \caption{Performance on edge cases from the VidSTG declarative test set. ``Overall'' refers to the full test set result in main paper.}                                        
\label{tab:edge_cases}                                                                                 \begin{tabularx}{\linewidth}{>{\raggedright\arraybackslash}X c c c c c c}                              
\toprule                                                  
% \rowcolor[gray]{0.95}                                                                                  
Setting & \#Samples & Avg. Len & m\_tIoU & m\_vIoU & vIoU@0.3 & vIoU@0.5 \\
\midrule                                                                                               
\rowcolor[gray]{0.9}                                                                                   
\textbf{Overall (Default)} & \textbf{4600} & \textbf{27.7s} & \textbf{52.6} & \textbf{37.2} & \textbf{52.4} & \textbf{37.4} \\                                                                     
\midrule                                                                                               
\multicolumn{7}{c}{\textit{\textcolor[gray]{0.5}{Video Duration}}} \\                                  
Short video ($<$3s)  & 13  & 2.9s   & 79.0 & 59.5 & 84.6 & 61.5 \\                                
Long video ($>$90s)  & 17  & 108.6s & 36.5 & 32.4 & 33.5 & 28.5 \\ 
\midrule      
\multicolumn{7}{c}{\textit{\textcolor[gray]{0.5}{Event Duration (Avg. Len = Avg. Time of Event Duration)}}} \\   
Short event ($<$1s)  & 366 & 0.7s  & 36.7 & 29.9 & 39.8 & 20.1 \\
\bottomrule                                                                          
\end{tabularx}
\end{table*}        

\subsection{Video Duration}
Bridge-STG performs strongly on short videos ($<$3s), achieving 79.0 m\_tIoU and 59.5 m\_vIoU—substantially higher than the overall performance (52.6 / 37.2).                              
The limited temporal span reduces ambiguity in event boundary prediction, allowing the model to focus on a compact temporal window.   

On long videos ($>$90s, avg. 108.6s), performance degrades to 36.5 m\_tIoU and 32.4 m\_vIoU, representing a 16.1-point drop in m\_tIoU and 4.8-point drop in m\_vIoU compared to the overall result.
This is consistent with our fixed 2 fps sampling strategy: for videos nearly 4$\times$ longer than the average (27.7s), the model must reason over a much longer sequence of frame pairs, making precise temporal boundary localization more challenging.                                                                                                                             

\subsubsection{Short Events}
Events with ground-truth durations shorter than 1 second (avg. 0.7s) present a significant challenge, with m\_vIoU dropping to 29.9 (a 7.3-point decrease) and vIoU@0.5 to only 20.1 ($-17.3$).
At 2 fps, a sub-second event may be captured by only 1--2 frames, leaving insufficient visual evidence for reliable spatial localization.                                                   
The larger drop in vIoU@0.5 compared to m\_vIoU indicates that while the model can still achieve coarse localization, precise grounding at the 0.5 IoU threshold becomes substantiall harder for such brief events.

\section{Qualitative Analysis}
We qualitatively compare our proposed Bridge-STG with an MLLM-based approach, LLaVA-ST, and a task-specific expert model, CG-STVG on VidSTG dataset for STVG task. The visualizations encompass both declarative and interrogative queries, which are further categorized into good cases (tIoU$\geq0.7$, vIoU$\geq0.5$ evaluated by our Bridge-STG) and bad cases (tIoU$\leq0.3$, vIoU$\leq0.2$ evaluated by our Bridge-STG). As illustrated across the visualizations, LLaVA-ST struggles to capture precise spatio-temporal details. Its decoder-free design leads to severely entangled spatio-temporal alignment, which is challenging to achieve precise spatial grounding of the target. This limitation is particularly pronounced in scenarios that identify the target referred to in short-duration actions and complex visual backgrounds, such as ``pull a motorcycle'' in Fig.~\ref{fig:intbad} and ``the baby being severely occluded'' in Fig.~\ref{fig:decbad}. In such challenging scenarios, our model exhibits robust localization boundaries, achieving overall performance on par with the task-specific expert model, CG-STVG. Notably, even within the identified bad cases, Bridge-STG still yields better quantitative spatio-temporal localization metrics compared to CG-STVG. These results underscore that the spatio-temporal semantic bridging mechanism within Bridge-STG effectively preserves rich temporal-aware characteristics and dynamic spatial information, which is pivotal for achieving fine-grained video understanding.

\section{Discussion}
\subsection{Limitation}
\noindent\textbf{Fixed Frame Sampling Rate.}
Bridge-STG uniformly samples frames at 2 fps, following standard practice in STVG~\cite{gu2024context, wang2025spacevllm}.
However, this fixed rate may be insufficient for videos containing rapid motion or fine-grained short-duration events (e.g., events shorter than 1 second), where critical visual cues can be missed between sampled frames.

\noindent\textbf{Cascaded Error Propagation.}
Bridge-STG adopts a sequential pipeline where spatial grounding is conditioned on the predicted temporal window $[t_\text{start}, t_\text{end}]$.
Consequently, inaccurate temporal localization directly limits the quality of spatial grounding, as QGSL only processes frames within the predicted window at inference time.

\noindent\textbf{Computational Overhead of Dual-Module Design.}
The decoupled architecture introduces an additional spatial decoder (QGSL) on top of the MLLM backbone, which increases the total parameter count.

\subsection{Future Work}
\noindent\textbf{Adaptive Frame Sampling.}
A natural extension is to replace fixed 2 fps sampling with adaptive strategies conditioned on motion magnitude or event density, enabling finer temporal resolution for fast-motion or short-duration events without increasing the total number of processed frames.

\noindent\textbf{Joint Temporal-Spatial Reasoning.}
The current sequential pipeline is susceptible to cascaded errors from temporal prediction.
Future work could explore joint temporal-spatial decoding mechanisms or iterative refinement strategies that allow spatial evidence to correct temporal predictions, improving robustness in ambiguous scenarios.

\noindent\textbf{Lightweight Decoder Design.}
To reduce the computational overhead of the dual-module architecture, future work could investigate knowledge distillation or parameter-efficient designs for the spatial decoder, enabling deployment in resource-constrained environments while preserving grounding accuracy.

\section{Code and Data Availability}
To maximize research impact and facilitate reproducibility, we commit to releasing all code, data, and models under permissive licenses upon the paper’s acceptance.

\section{Ethical Considerations}
All datasets used in this work are publicly available academic benchmarks released under standard research licenses.     
Specifically, VidSTG~\cite{zhang2020does} and HC-STVG~\cite{tang2021human} are derived from the VidOR and publicly available video sources; Charades-STA~\cite{gao2017tall} is built upon the Charades dataset collected with informed participant consent.
GOT-10K~\cite{huang2019got} consists of publicly available video footage.
And RefCOCO/RefCOCO+/RefCOCOg~\cite{kazemzadeh2014referitgame, mao2016generation} are derived from MS COCO images~\cite{lin2014microsoft}.                                             
The self-collected training data is synthesized entirely from REVOS~\cite{yan2024visa}, a publicly released video object segmentation dataset, through an automated construction pipeline.  
No new videos are recorded, no human subjects are recruited, and no additional annotations are crowd-sourced.                                                                             
All synthetic samples are derived solely from existing publicly available annotations.
No personally identifiable information is collected, stored, or processed in this work.
The proposed Bridge-STG model is designed for video understanding research and does not introduce new capabilities for surveillance, tracking of individuals without consent, or other potentially harmful applications.
We encourage responsible use of this work in accordance with applicable laws and ethical guidelines. 

% %%
% %% The next two lines define the bibliography style to be used, and
% %% the bibliography file.

\bibliographystyle{ACM-Reference-Format}
\bibliography{sample-base}

\clearpage

\begin{figure*}
  \includegraphics[width=\textwidth]{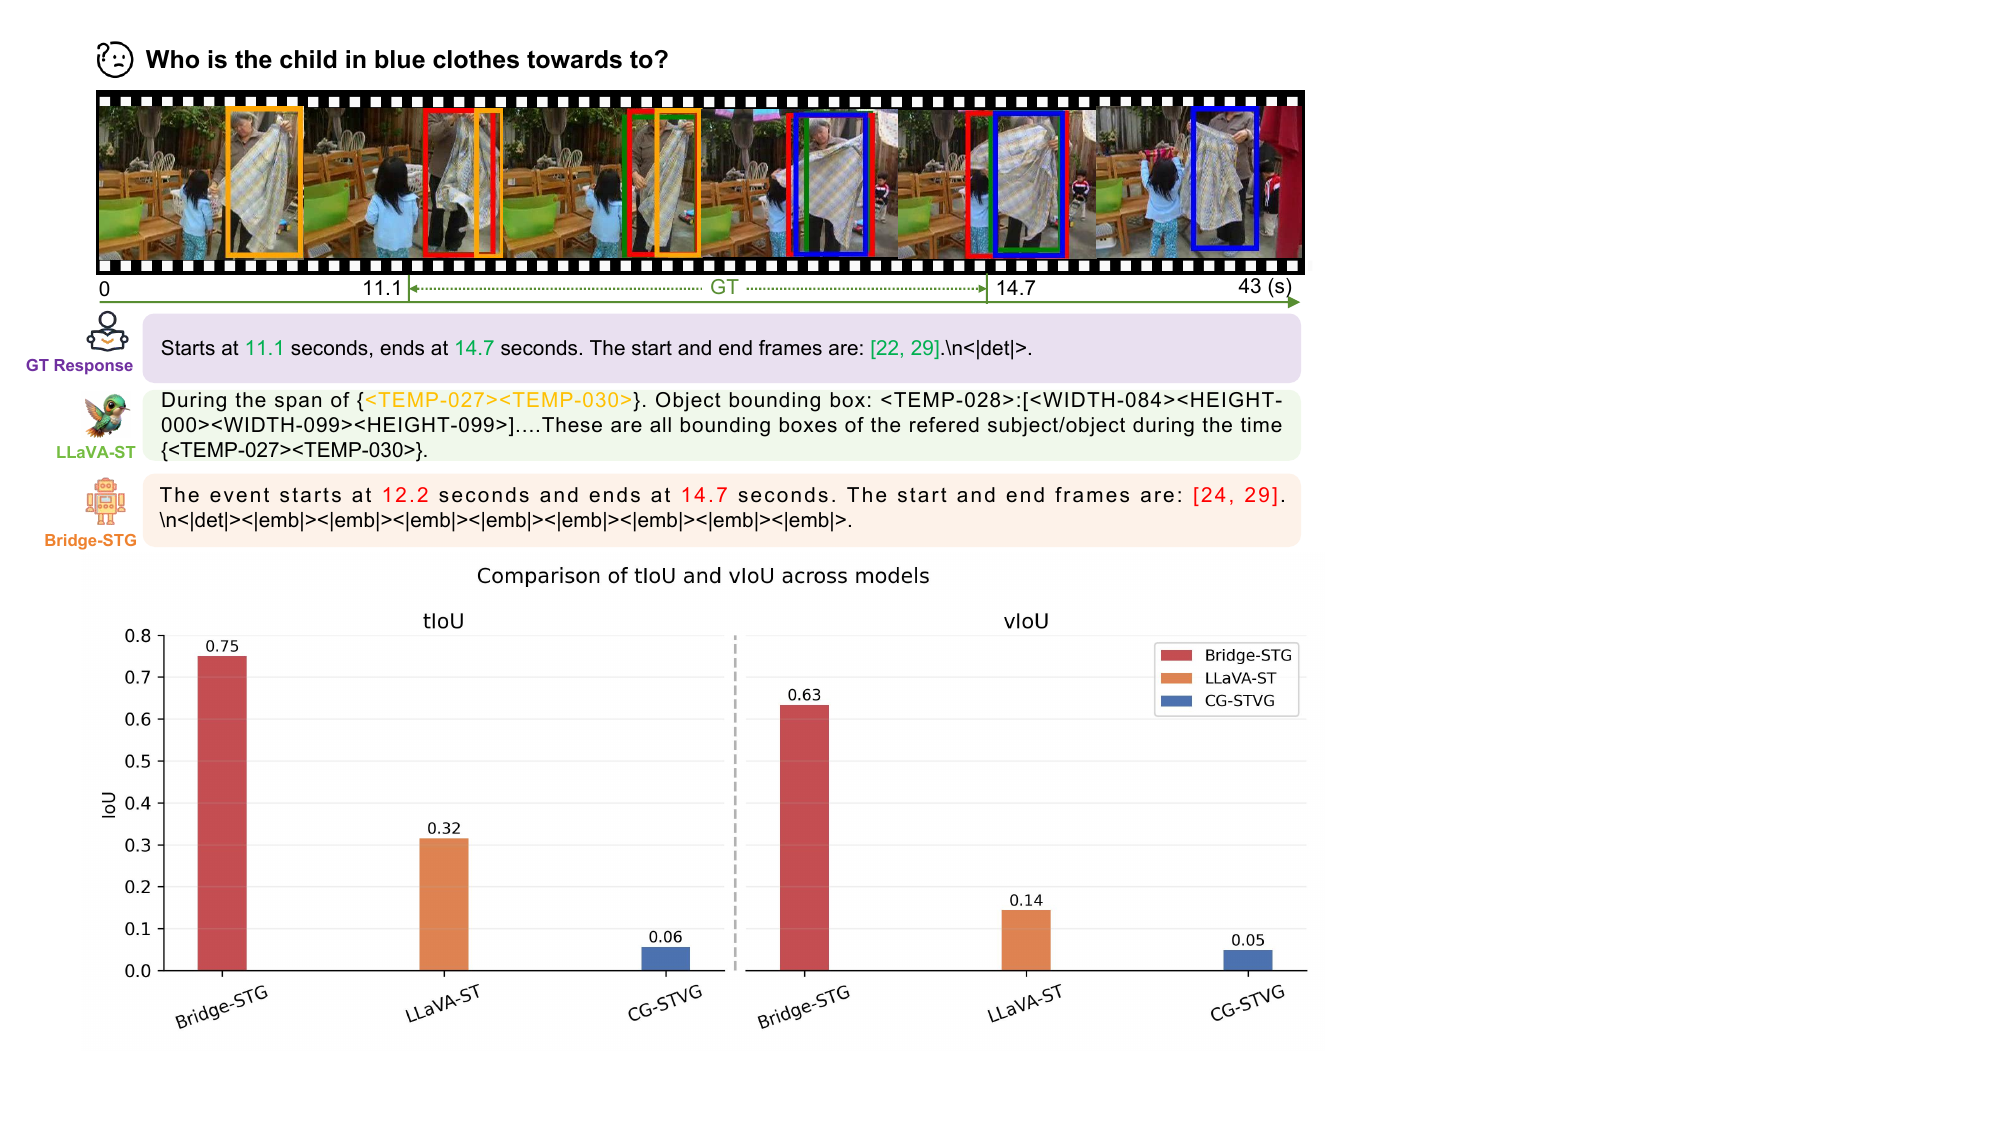}
  \caption{Visualization of good case on VidSTG interrogative test subset between different model for STVG task.
 As the box in the video, \textcolor{green}{green} represents ground-truth bounding box, \textcolor{blue}{blue} is the CG-STVG, \textcolor{orange}{orange} is LLaVA-ST and \textcolor{red}{red} is our Bridge-STG.}
  \label{fig:intgood}
\end{figure*}

\begin{figure*}
  \includegraphics[width=\textwidth]{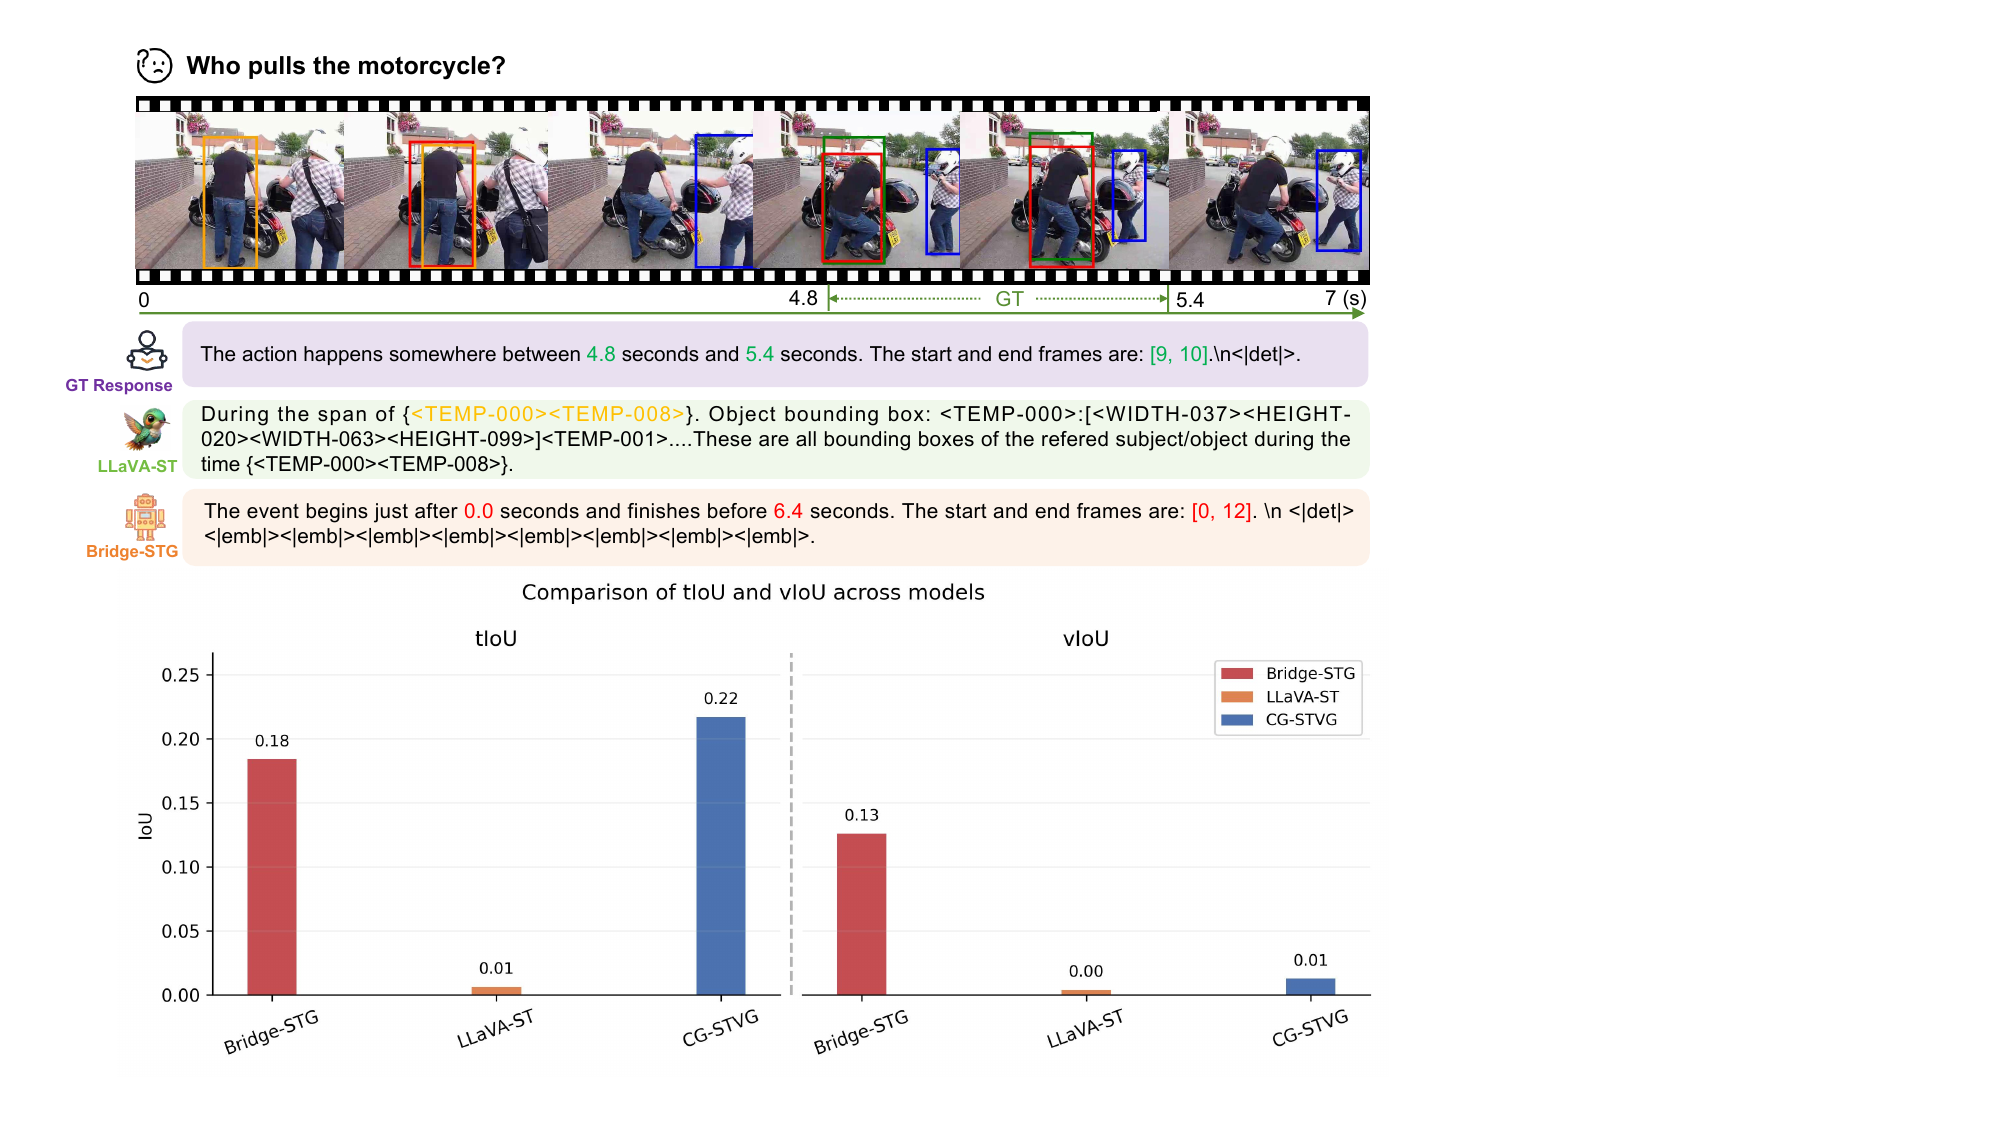}
  \caption{Visualization of bad case on VidSTG interrogative test subset between different model for STVG task.}
  \label{fig:intbad}
\end{figure*}

\begin{figure*}
  \includegraphics[width=\textwidth]{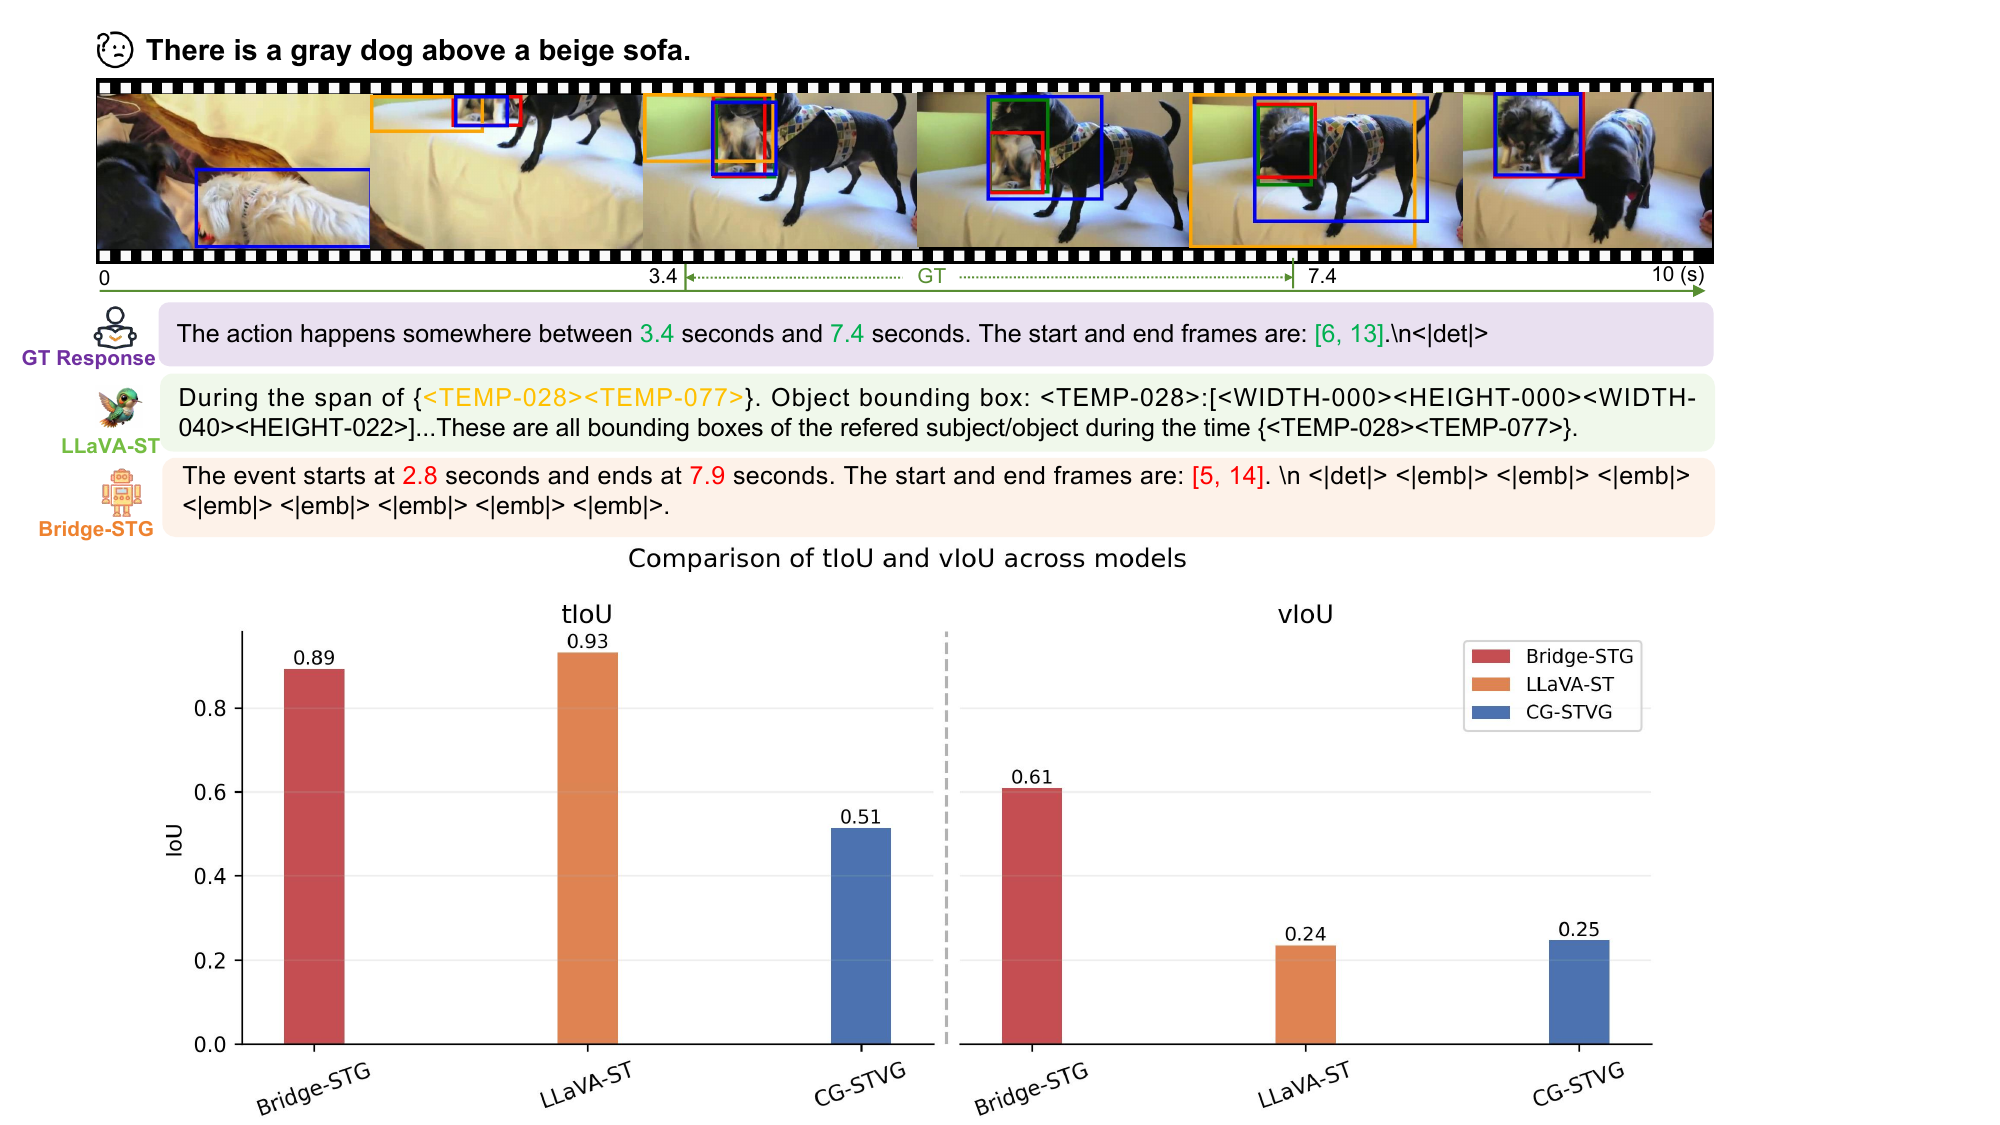}
  \caption{Visualization of good case on VidSTG declarative test subset between different model for STVG task.}
  \label{fig:decgood}
\end{figure*}

\begin{figure*}
  \includegraphics[width=\textwidth]{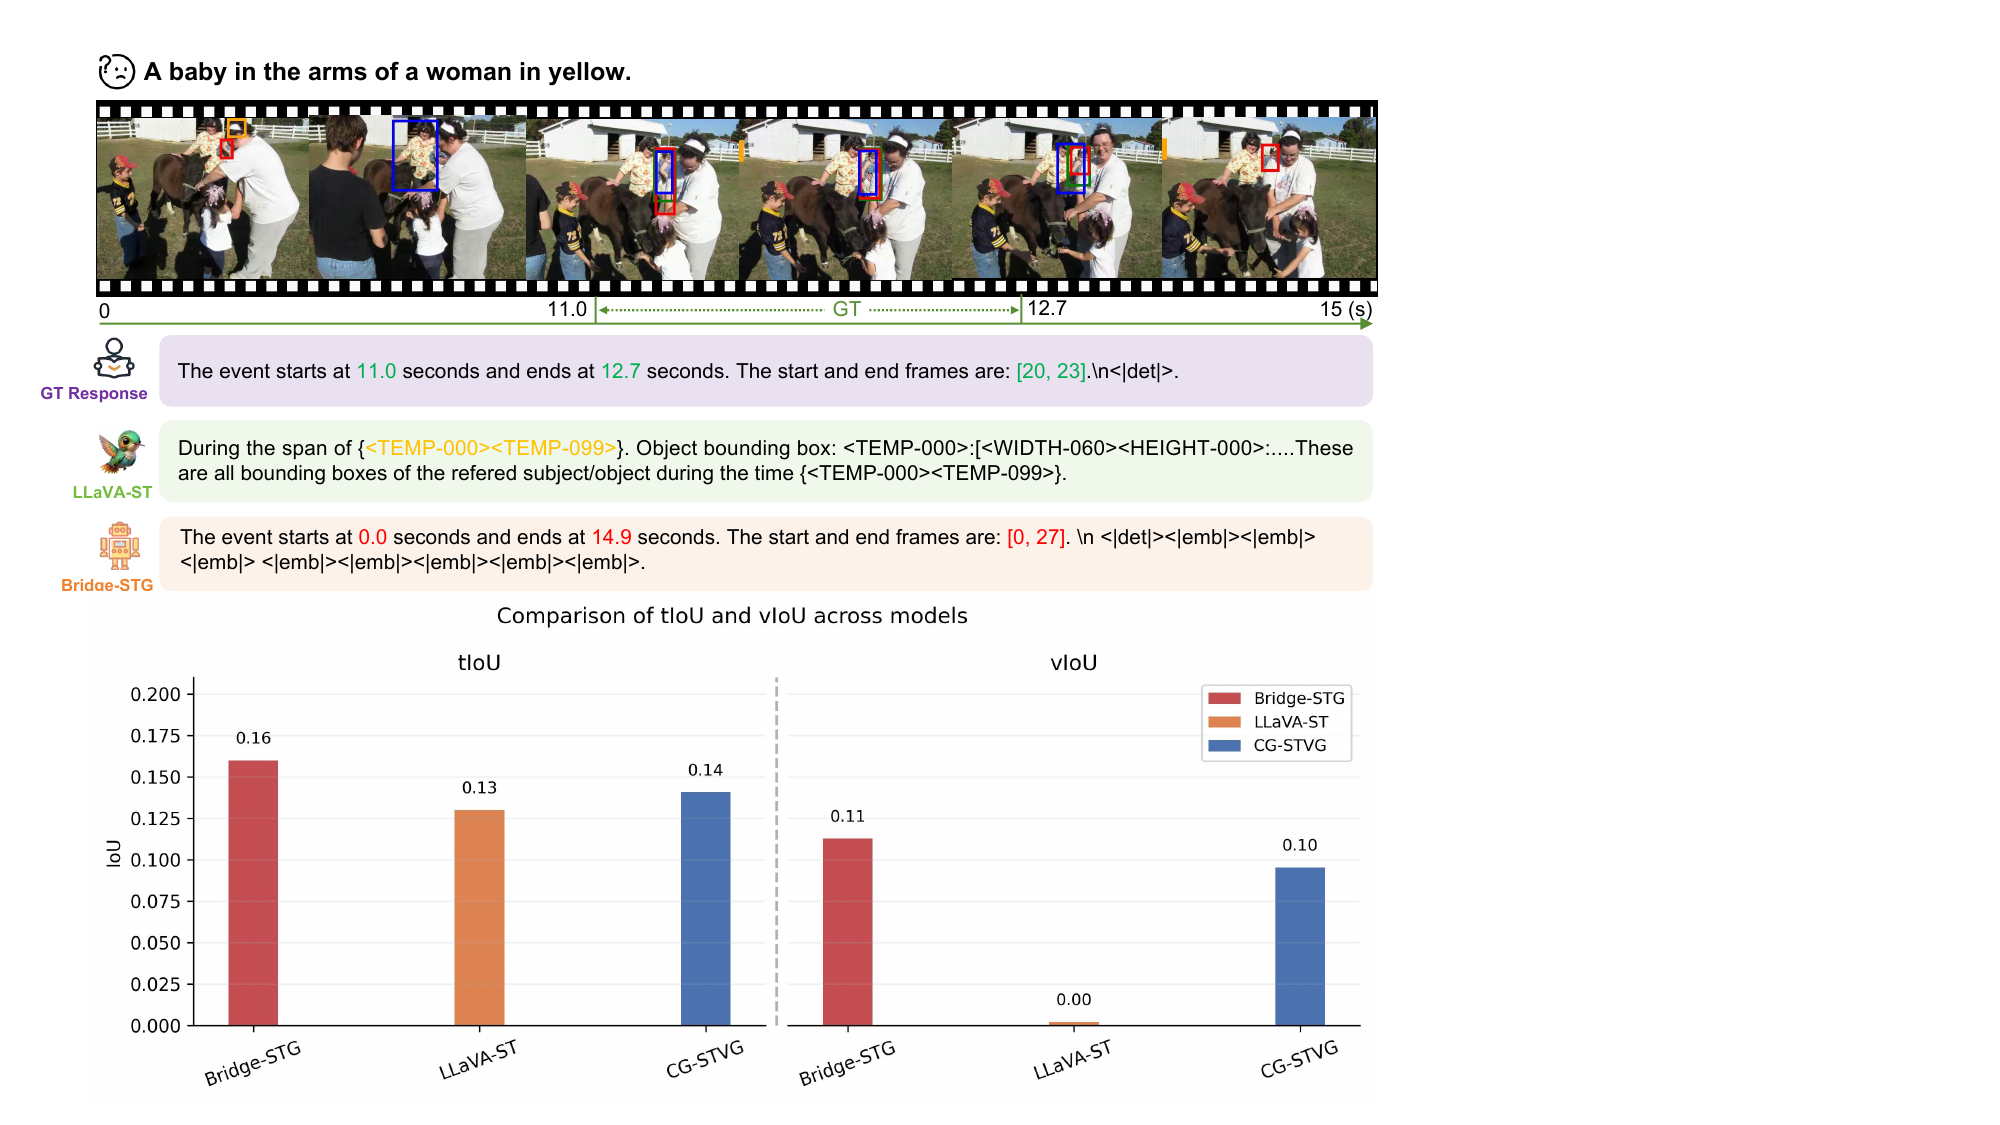}
  \caption{Visualization of bad case on VidSTG declarative test subset between different model for STVG task.}
  \label{fig:decbad}
\end{figure*}

% %%
% %% If your work has an appendix, this is the place to put it.

% \section{Research Methods}

% \subsection{Multi-Layer Interactive Queries}
% \subsubsection{Number of layers}
% \subsubsection{Advantages of multi-level query compared to the single-level query}

% \subsection{Image-Query Alignment}
% \subsubsection{$L_{align}$}

% \subsubsection{$L_{dn}$}

% \section{Visualization Results}

\end{document}
